# Supplementary material for: Spin filter for arbitrary spins by substrate engineering
Source: arXiv:1604.01520 ancillary file (2016-07-31)
Supplement: Supplementary file 1 [file supplemental.pdf]

# Spin filter for arbitrary spins by substrate engineering: supplemental material

Biplab Pal,<sup>1,\*</sup> Rudolf A. Römer,<sup>2,†</sup> and Arunava Chakrabarti<sup>1,‡</sup>

<sup>1</sup>*Department of Physics, University of Kalyani, Kalyani, West Bengal-741235, India*

<sup>2</sup>*Department of Physics and Centre for Scientific Computing,  
University of Warwick, Coventry, CV4 7AL, UK*

In this supplemental material we present the figures for higher spin states – both for the constant values of the polar angle  $\theta$  as well as for a ‘spiral’ configuration in  $\theta$ . These results are complementary to the results discussed in the main paper. The methods and mathematical framework we have used to obtain these results are already discussed in the main paper.

happens for the spin-2 case as well but we have refrained from exhibiting those figures here since the main idea is easily understood from the results of the spin-1 case. For spin-3/2, the phenomena of spin flipping happens as well and a particle with a certain spin component flips to its counter part.

## I. CONSTANT POLAR ANGLE $\theta$

In this section we present the results for constant polar angle  $\theta$ . In Fig. S1 we show the local density of states (LDOS) and the corresponding two terminal transmission coefficient for a fixed  $\theta = \pi/4$  and for different values of the strength of the magnetic moment  $h$ . This figure is the counter part of Fig. 4 in the main text for non-zero value of  $\theta$ . In Fig. S2 and Fig. S3 we have exhibited a similar analysis corresponding to the spin-3/2 and spin-2 cases for  $\theta = 0$ . These two figures are complementary to the Figs. 2 and 4 given in the main article but now for higher spin states. Here we have a larger number of bands corresponding to different spin channels as the number of spin components has increased. The central idea remains the same as discussed in the main paper for spin-1/2 and spin-1 cases.

## II. SPIRAL CASES

In Fig. S4, and Fig. S5 we show results for the LDOS and transmission characteristics corresponding to spins  $S = 1$  and  $S = 3/2$ , respectively, for a *spiral* configuration of the local magnetic moments. These two figures are in the connection to Fig. 7 in the main paper. Similar to the main paper, here also we get a spin flip transmission for a half period in the spiral configuration in the orientation of the local magnetic moments as compared to system length, and the phenomenon of spin flipping disappears for full period in spiral as compared to the system size. For the spin-1 case, the central spin channel corresponding to the spin-0 component does not exhibit this feature of spin flipping as  $h$  has no role to play for the spin-0 component. We have verified that the same thing

---

\*Electronic address: [biplabpal@klyuniv.ac.in](mailto:biplabpal@klyuniv.ac.in)

†Electronic address: [r.roemer@warwick.ac.uk](mailto:r.roemer@warwick.ac.uk)

‡Electronic address: [arunava.chakrabarti@yahoo.co.in](mailto:arunava.chakrabarti@yahoo.co.in)

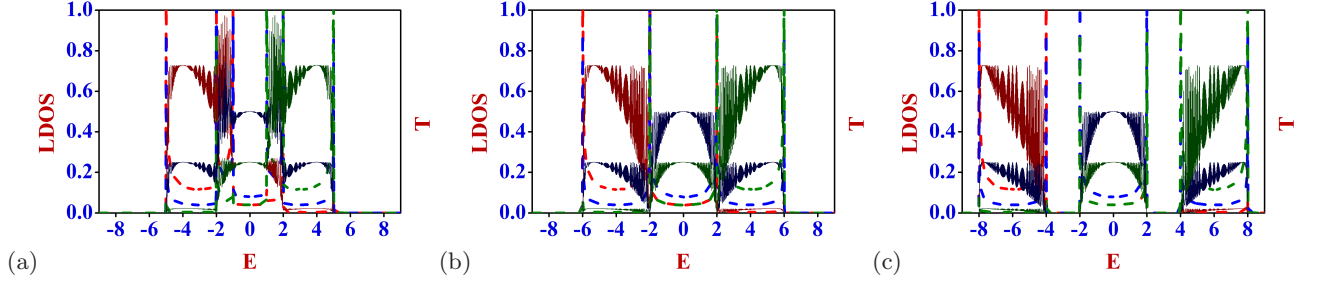

FIG. S1: (Color online) Variation of LDOS and transmission probabilities with energy  $E$  as a function of  $h$  for a fixed value of  $\theta = \pi/4$  for spin-1 particles. The curves with the red dashed line represent the LDOS for the spin-1 states, the curves with the blue dashed line represent the LDOS for the spin-0 states, and the curves with the green dashed line represent the LDOS for the spin-(-1) states. The dark red curve represents the transmission probability for the spin-1 particles, dark blue curve represents the transmission probability for the spin-0 particles, the dark green curve is exhibiting the transmission probability for the spin-(-1) particles. (a) is for  $h = 3$ , (b) is for  $h = 4$ , and (c) corresponds to  $h = 6$ . The lead parameters for the non-magnetic leads are  $\epsilon_L = \epsilon_R = 0$  and  $t_{LD} = t_{RD} = t_L = t_R = 4$ .

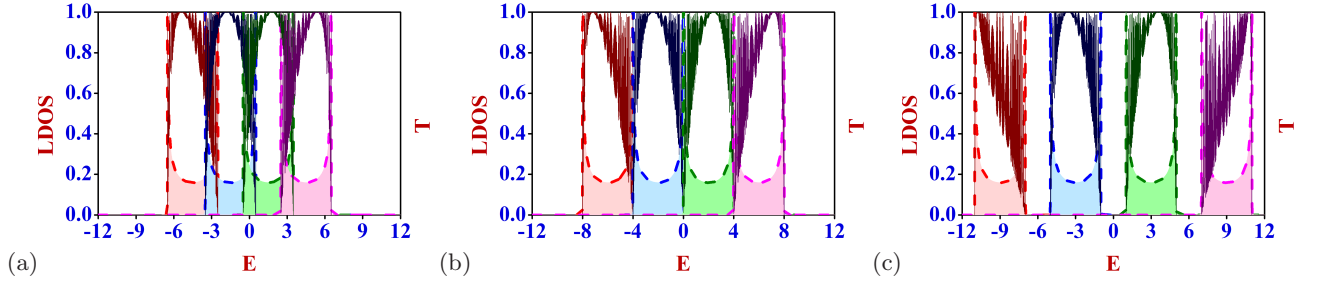

FIG. S2: (Color online) Variation of LDOS and transmission probabilities with energy  $E$  as a function of  $h$  for a fixed value of  $\theta = 0$  for spin-3/2 particles. The light red shaded plot with the dashed red envelope is the LDOS for the spin-3/2 states, the light blue shaded plot with the blue dashed envelope is the LDOS for the spin-1/2 states, the light green shaded plot with the green dashed envelope is the LDOS for the spin-(-1/2) states, and the light magenta shaded plot with the magenta dashed envelope is the LDOS for the spin-(-3/2) states. The dark red curve represents the transmission characteristics for the spin-3/2 particles, the dark blue curve is for the spin-1/2 particles, the dark green curve is for the spin-(-1/2) particles, and the dark magenta curve is for the spin-(-3/2) particles. (a) is for  $h = 4.5$ , (b) is for  $h = 6$ , and (c) corresponds to  $h = 9$ . The lead parameters for the non-magnetic leads are  $\epsilon_L = \epsilon_R = 0$  and  $t_{LD} = t_{RD} = t_L = t_R = 6$ .

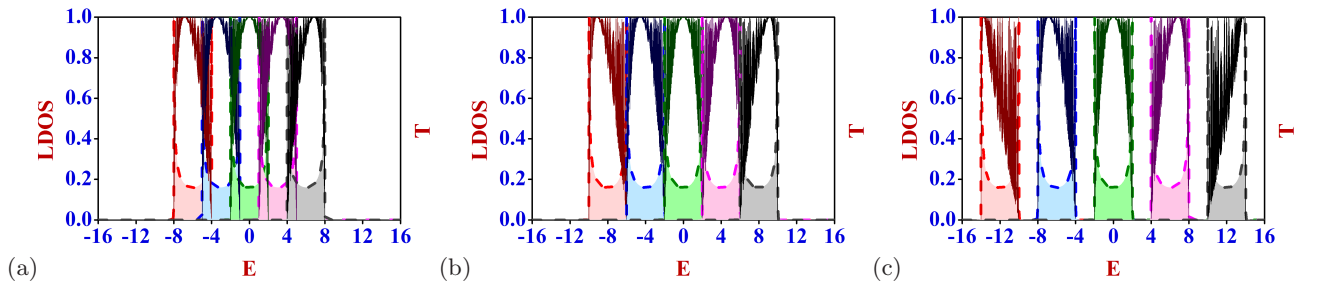

FIG. S3: (Color online) Variation of LDOS and transmission probabilities with energy  $E$  as a function of  $h$  for a fixed value of  $\theta = 0$  for spin-2 particles. The light red shaded plot with the dashed red envelope is the LDOS for the spin-2 states, the light blue shaded plot with the blue dashed envelope is the LDOS for the spin-1 states, the light green shaded plot with the green dashed envelope is the LDOS for the spin-0 states, the light magenta shaded plot with the magenta dashed envelope is the LDOS for the spin-(-1) states, and the light gray shaded plot with the dark gray dashed envelope is the LDOS for the spin-(-2) states. The dark red curve represents the transmission characteristics for the spin-2 particles, the dark blue curve is for the spin-1 particles, the dark green curve is for the spin-0 particles, the dark magenta curve is for the spin-(-1) particles, and the black curve is for spin-(-2) particles. (a) is for  $h = 6$ , (b) is for  $h = 8$ , and (c) corresponds to  $h = 12$ . The lead parameters for the non-magnetic leads are  $\epsilon_L = \epsilon_R = 0$  and  $t_{LD} = t_{RD} = t_L = t_R = 8$ .

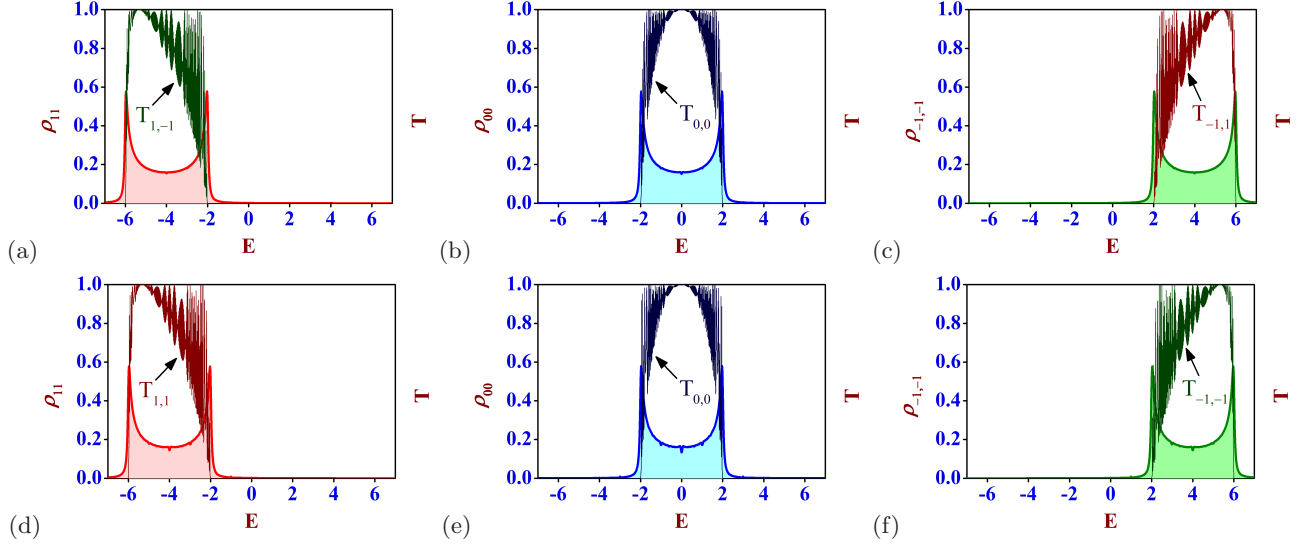

FIG. S4: (Color online) Plot of LDOS and transmission probabilities for spin-1 particles for spiral configurations of the magnetic moments in the magnetic chain system. The figures in the top panel [(a), (b) and (c)] are for a variation of the angle  $\theta_n = n\pi/L$ , and the figures in the bottom panel [(d), (e) and (f)] correspond to an angle variation  $\theta_n = n\pi/(L/2)$  with  $L = 300$ . We have set  $h = 4$  for all the magnetic sites in the chain.

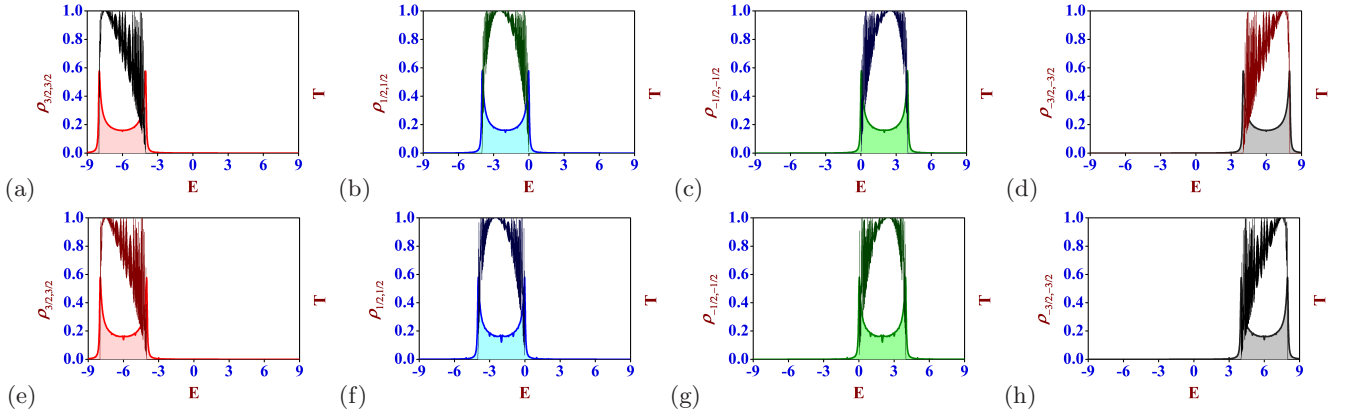

FIG. S5: (Color online) Plot of LDOS and transmission probabilities for spin-3/2 particles for spiral configurations of the magnetic moments in the magnetic chain system. The figures in the top panel [(a), (b), (c) and (d)] are for a variation of the angle  $\theta_n = n\pi/L$ , and the figures in the bottom panel [(e), (f), (g) and (h)] correspond to an angle variation  $\theta_n = n\pi/(L/2)$  with  $L = 300$ . We have set  $h = 6$  for all the magnetic sites in the chain.
